# Supplementary material for: ARAPReg: An As-Rigid-As Possible Regularization Loss for Learning Deformable Shape Generators
Source: arXiv:2108.09432 source file (2021-09-21)
Supplement: Supplementary file 1 [file 08_appendix.tex]

\section{Formulation for the Derivative}

Note that 
$$
H = L\otimes I_3  - A^T D^{-1} A.
$$

$$
dH = - dA^T D^{-1} A - A^T D^{-1} dA + A^T D^{-1} dD D^{-1}A.
$$
